# Supplementary material for: Trenchcoat: Human-Computable Hashing Algorithms for Password Generation
Source: arXiv:2310.12706 source file (2023-10-19)
Supplement: Supplementary file 1 [file backup-appendix.tex]

\subsection{Collision resistance}

In our case, an adversary cannot even compute or verify $h_R$ efficiently, since $R$ is unique to each individual. In that sense, our hash function is similar to a physically unclonable function~\cite{suh2007physical}. Although the incidence of collisions should be rare and hard to find, we formalize this as:
For all  $y \in h_R$ (i.e., the range) and $m \in M$, where $\epsilon$ is negligible, and $M$ is the set of all secrets parameterized by website name, and $n$ are the number of trials of the function, the following computations are infeasible with a probabilistic polynomial time algorithm; $3 \implies 2$ and $1$:
\begin{itemize}
    \item [1] One way functions: given a password $y$, we guess $m$. $P(h_R(m) = y) \leq \epsilon = {2^{-78}}$ in the average case (length 11.83), as analysed at the end of section~\ref{sec:subuserstudy}.
    \item [2] Weakly collision-free: Given an $m$, we guess $m^\prime  \in M$, \\ $P(h_R(m^\prime) = h_R(m) \text{ and } m^\prime \neq m)  \leq \epsilon = {2^{-78}}$, but this case is also unrealistic, since the adversary cannot even compute the hash function.
    \item [3] Strongly collision-free: The adversary guesses a pair of messages $m$ and $m^\prime$. Here as well, one would get the usual bound for $P( h_R(m^\prime) = h_R(m))$, with the addendum that the adversary cannot compute even one hash to confirm, meaning that the real bound is actually the full range of possible outputs.
\end{itemize}

The Memory Palace algorithm is weakly collision resistant\footnote{$h_R$(shopsentence, user1) $\longrightarrow$ a1e3xdhusehu, and \\ $h_R$(loadsentence,user1) $\longrightarrow$ a1e3xdhusehu (with fixed sources of randomness assuming the same user generating each subkey. Subkeys were generated using a random word generator from a dictionary of the 3000 most common English words ~\cite{press})}, however the collision rate is extremely low ($<0.001$) and in practice is lower for passwords created by different users. Collisions occurred with a high number of passwords generated by the same user which is improbable in reality. It is also impossible to predict subkeys that users generate, and highly unlikely that two subkeys are similar due to the priming instructions within the algorithm. Usage of languages other than English also contributes to a low collision incidence.

No incidences of collision were present in the Song Password, Scrambled box and Cue Pin Select methods except in instances where users disregarded instructions. Some collisions were present in same-user Cue-Pin-Select passwords.


\subsection{Randomness} \label{sec:randomness}
Apart from sources of randomness mentioned in section \ref{sec:hashing}, we note one small addition for methods such as Song Password and Memory Palace that map alphabets to sets of numbers: whether letters are indexed from 0 or 1. 

The interpretation of diagonal keys on a keyboard are also a source of randomness. Interpretations of the angle of diagonal differ between users and the choice of whether to use the diagonal character in the first row above a character, second row etc also vary. These rules are intentionally vaguely defined; users naturally derive a specific meaning and stick to it, based on their $R$. It is also observed that users in real-life use a mix of local languages as well as English to describe locations familiar to them, which results in better passwords.

Another approach to measuring randomness in a hash function is to measure the change in the hash corresponding to changes in inputs. For true randomness, half of the hash must change for every change of 1 hamming distance in the input. For example, given two strings that are 1 hamming distance apart, ‘aaa’ and ‘aab’, a SHA3-256 hash produces outputs that have 4/64  identical characters in terms of position and sequence. However this analysis is unfeasible on any human-computable hash functions as it is almost impossible that input strings - keys- are only one hamming distance apart when users create them, and they cannot be controlled for. 
Using memory palace $h_R(Store) = mkgyw3$ and $h_R(stove) = mkkow3$, given either (key,hash) pair adversaries may deduce that $m$ maps to $st$, $g$ maps to $or$ and $w$ maps to  $e$; in the second hash $g$ is replaced by $k$, in which case adversaries can use a dictionary of words with $St \_ \_e$. However in reality users used $h_R(shoe store) = c(o9i7$ and $h_R(Stove) = Xgkgs$ and were able to partially and completely (respectively) recollect their passwords.

Words occuring in subkeys for the Memory Palace are also uncommon, with only 4\% of \textit{partial words} in subkeys found in the 100 most common words in English. We note that revealing one subkey does not reveal other subkeys, as each user's visual navigation and associative memories are distinctive. 

We refer readers to \cite{CuePinSelect} for a detailed analysis of the security of Cue-Pin-Select.

%end
